# Supplementary material for: MEFLUT: Unsupervised 1D Lookup Tables for Multi-exposure Image Fusion
Source: arXiv:2309.11847 source file (2023-09-21)
Supplement: Supplementary file 1 [file supp.tex]

% As seen in Fig.~\ref{fig:our_vis4}, the results of the other methods commonly fail to recover the details of saturated regions in the coat hanger. In contrast, our method hallucinates more accurate contents in over saturated areas, causing the pattern of clothes better preserved. 
% % As seen in Fig.~\ref{fig:our_vis_su1}, 
% In Fig.~\ref{fig:our_vis_su1}, the results of the other methods recover less details in the overexposed areas of the night light, while our method can preserve more accurate details in over saturated areas. 
% %As seen in Fig.~\ref{fig:our_vis_su2}, 
% It can be seen in Fig.~\ref{fig:our_vis_su2} that the results of the other methods fail to  recover details in the overexposed area of the sign at night, while our method can recover accurate contents, causing the clear sign details. 

% \section{More Comparision with other Methods on SICE Test Set}
% We also compare our method with 6 previous MEF methods on SICE dataset. Comparision results show in Fig.~\ref{fig:sice_vis2}. the results of the other methods commonly fail to recover the details of saturated regions in the edge of porch. In contrast, our method hallucinates more accurate contents in over saturated areas, causing the clear details.

\section{More Details of Our Ablation Studies}
% \vspace{-2mm}
\paragraph{Comparison with other phones.} 
We compared the results with some MEF methods in the existing smartphones. Two flagship phones of XiaoMi and Honor are applied as comparisons. As shown in Fig.~\ref{fig:our_rebuttal}(b) and (d), they are the results for other smartphones brands, and Fig.~\ref{fig:our_rebuttal}(a) and (c) are the results of our method ported to smartphones. Our method has better results in the details of the sky and buildings.

% \input{./include/tab-validity.tex}

% color degradation
% \subsubsection{Robustness of 1D LUTs.}
% \paragraph{Trained network vs. LUTs.} Although the LUTs in our method do not participate in the training. As shown in Tab.~\ref{table:lut_gap}, we find that the quality of the results of the LUTs is basically similar to that of the trained network, but the speed is several times faster. If using a network to predict weights, the weights may be smoother when the context information exists, but we find that it has little effect in actual deployment, and using LUTs will get a large speed advantage with less quality loss. Meanwhile, GFU has the ability to aggregate context information, and will make some supplements to the context information.

\paragraph{Robustness of arbitrary number inputs.}
Our technical design is not only unique, but also flexible to support the arbitrary number of exposure inputs. In real application scenarios, we notice that the number of input frames is sometimes not equal to the number of LUTs we provided. If the number of the input frames is less than the number of LUTs, we use some existing sequence extension methods~\cite{ipol.2019.278} to expand the inputs to the same number of LUTs. Then, if the number of input frames is more than the number of LUTs provided, we divide the inputs into groups with the same number of LUTs, and then average the frames within the group. In Tab.~\ref{table:mutil_frame_test} we use the above method to carry out experiments with three 1D LUTs and the different numbers of input frames. Experiments show that our method achieves good results even if the number of input frames is different from the number of LUTs.
% \vspace{-2mm}
% \vspace{-0.7cm}
% \paragraph{Robustness of 1D LUTs.}

\paragraph{Pyramid blending vs. Linear blending.} Using a multi-resolution scheme to blend the images is also suitable for our method and can acquire better results, but the speed is much slower than ours. Our method can satisfy the use of low-performance platforms. Tab.~\ref{table:linear} shows the comparison.

 \begin{figure}[ht]
   \centering
   \includegraphics[width=1.0\linewidth]{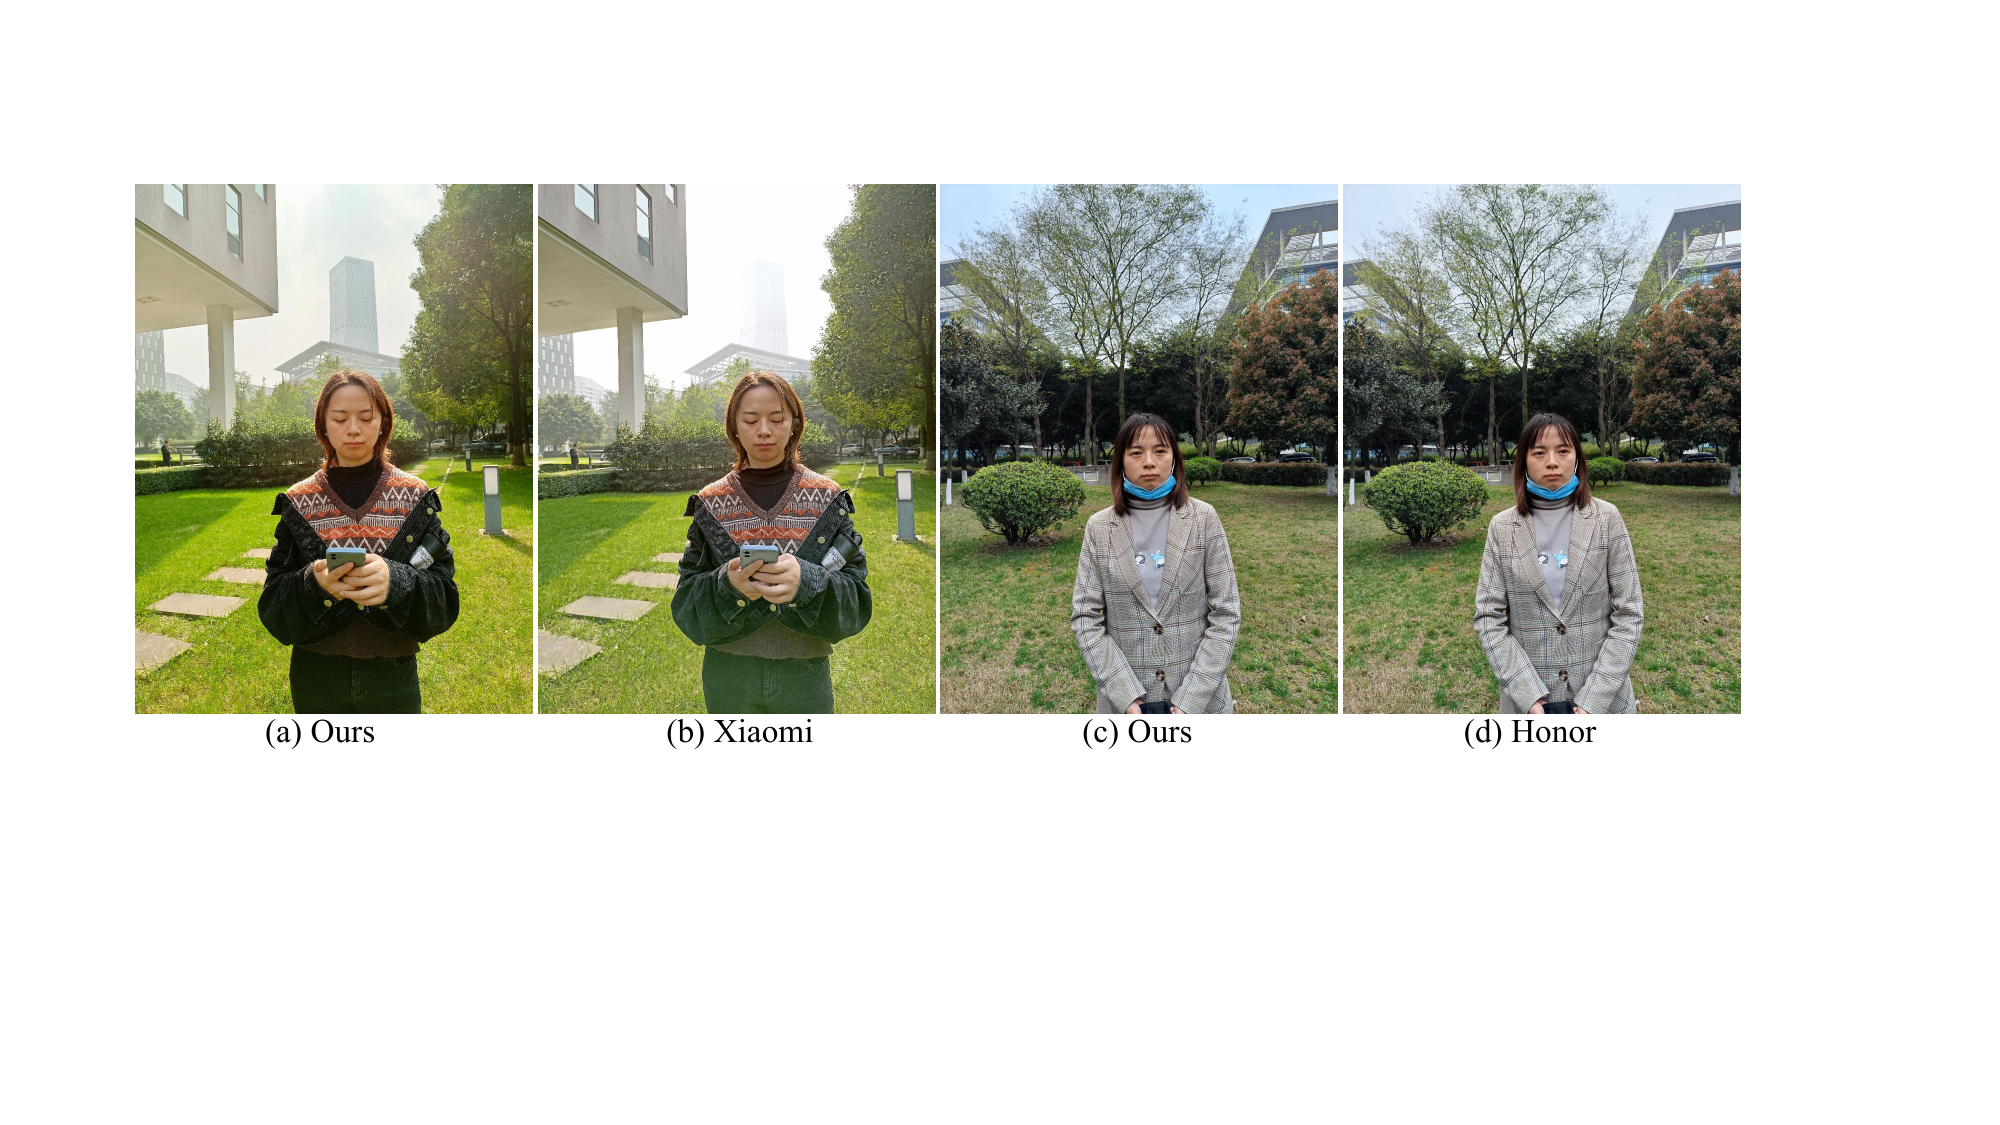}
   \caption{Qualitative comparison of the proposed method with other method in the existing smartphones, our method hallucinates more reasonable details in saturated regions.
   } \label{fig:our_rebuttal}
   \vspace{-3mm}
 \end{figure} 
\begin{figure}[t]
    \centering
    \includegraphics[width=0.86\linewidth]{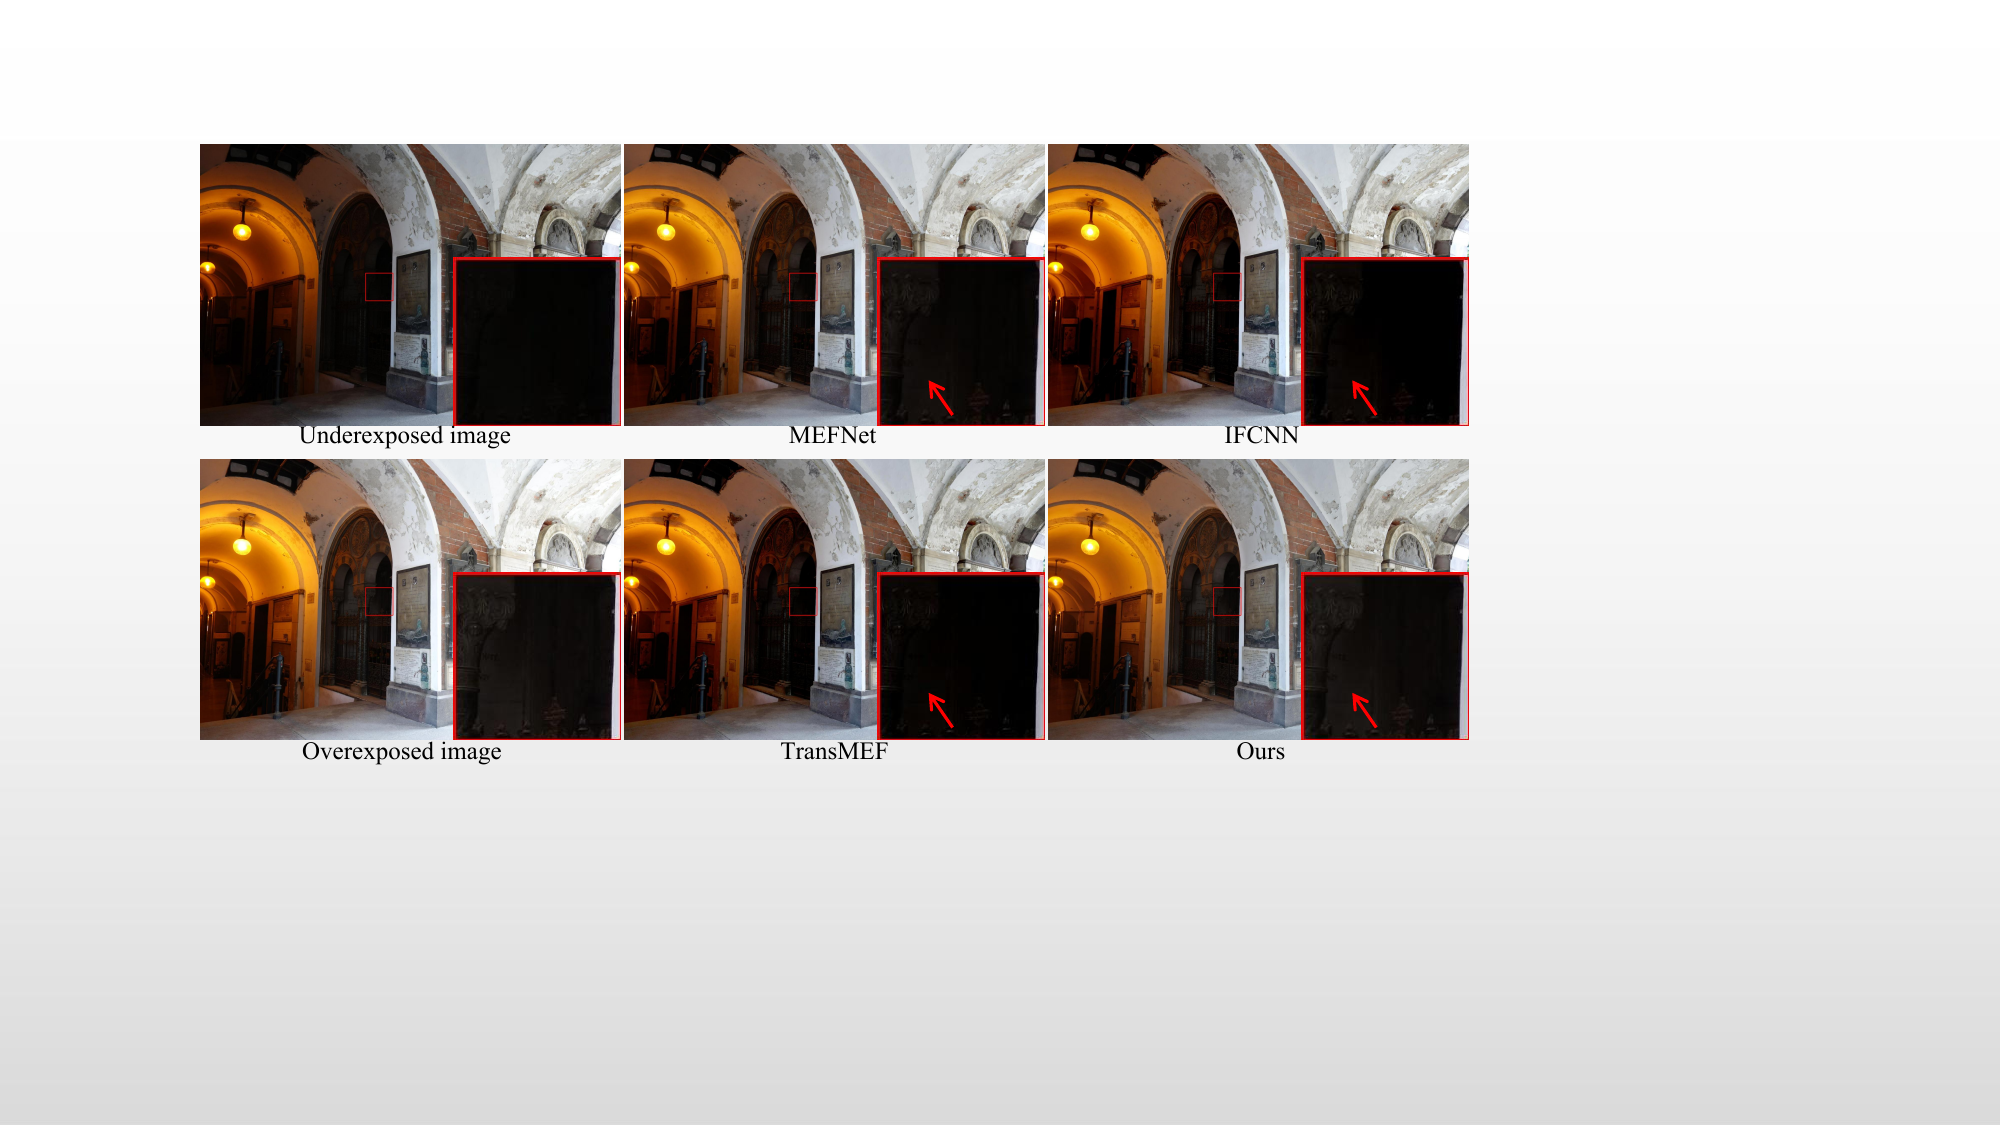}\vspace{-4mm}
    \caption{Visual comparison with several state-of-the-art methods in dark regions, as indicated by the red arrow.
  }\vspace{-3mm}
  \label{fig:dark}
\end{figure}
\paragraph{Dark regions:} We further compare the dark regions with some recent methods. Fig.~\ref{fig:dark} shows a visual example, where we acquire best dark regions details.

\begin{table}[t]
    \centering
    
    \setlength{\tabcolsep}{8.0 pt}
    \resizebox*{0.98\linewidth}{!}{
    \begin{tabular}{cccccc}
    \toprule
             \multirow{2}*{Metrics}& \multicolumn{5}{c}{Exposure Number ($K$)}   \\ \cline{2-6}
             & 2 & 3 & 4 & 5 & 6 \\ \hline
    PSNR$\uparrow$     & 31.016   & \textbf{31.387} & 31.253    & 30.858   & 30.525   \\ 
    SSIM$\uparrow$     & 0.9528   & \textbf{0.9590}      & 0.9532    & 0.9473    & 0.9432   \\ 
    Q$_\emph{C}$ $\uparrow$  & 0.6024 & \textbf{0.6075} & 0.6013 & 0.5981 & 0.5874\\ 
    MEF-SSIM$\uparrow$ & 0.9669   & \textbf{0.9688}     & 0.9686    & 0.9683     & 0.9656  \\
    \bottomrule
    \end{tabular}}
    \vspace{1mm}
    \caption{Robustness experiment based on three 1D LUTs and the arbitrary number of exposure inputs. The best results being highlighted in bold.}
    \label{table:mutil_frame_test}
    \vspace{-3mm}
\end{table}

\begin{table}[t]
  \centering
  \resizebox{0.86\linewidth}{!}{
  \setlength{\tabcolsep}{11 pt}
  \begin{tabular}{c|ccccc}
    \toprule %添加表格头部粗线
    Methods  & PSNR$\uparrow$ & SSIM$\uparrow$ & Q$_C$$\uparrow$ & MEF-SSIM$\uparrow$ & Running time (ms) \\
    \hline
     Multi-resolution & \textbf{31.412} & \textbf{0.9621} & \textbf{0.6096} & \textbf{0.9714} & 304.50 \\
     Ours & 31.387 & 0.9590 & 0.6075 & 0.9688 & \textbf{12.75} \\
    \bottomrule
  \end{tabular}}
  \vspace{-3mm}
  \caption{Comparison experiments with the multi-resolution scheme. The running platform is Mobile CPU ($K=3$).}
  \label{table:linear}
  \vspace{-3mm}
\end{table}
\begin{table}[t]
  \small
    \centering
    % \setlength{\tabcolsep}{2.0 pt}
    % % \vspace{-2mm}
\resizebox*{0.98\linewidth}{!}{
\setlength{\tabcolsep}{1.5 pt}
  \begin{tabular}{cccccc}
    \toprule %添加表格头部粗线
    Variants & PSNR$\uparrow$  & SSIM$\uparrow$ & Q$_C$$\uparrow$ & MEF-SSIM$\uparrow$ & Running Time (ms)\\
    \hline
    %   PSNR & 31.189 &  \textbf{33.941} \\
    %   SSIM & 0.9648 & \textbf{0.9691} \\
    %   MEF-SSIM & 0.9678 & \textbf{0.9692} \\
    %   Running Time (ms)&  \textbf{1.51} & 3.54 \\
    BU & 29.189 & 0.9548 & $0.6052$& 0.9674 & \textbf{0.95} \\
    GFU & \textbf{31.387} & \textbf{0.9590} &  $\textbf{0.6075}$&\textbf{0.9688} & 3.54 \\
    % w/o. GFU & \textbf{31.387} & \textbf{0.9590} &  $\textbf{0.6075}$&\textbf{0.9688} & 3.54 \\
    \bottomrule
  \end{tabular}}
  % \vspace{-2mm}
 \caption{The effectiveness of GFU, tested under $K=3$. BU denotes the Bilinear upsampling. The best results being highlighted in bold.}
\label{table:diff_up}
\vspace{1mm}
\resizebox{0.98\columnwidth}{!}{
    \setlength{\tabcolsep}{8 pt}
    \begin{tabular}{c|cccc}
    \toprule
    %     & PSNR$\uparrow$  & SSIM$\uparrow$ & \emph{Q}$_\emph{C}$ $\uparrow$ \\
    % \hline
    %     Mertens09 [8] & 31.547    & 0.8851 & 0.3412  \\
    %     Li13 [11]      & 20.133  & 0.8450 & 0.3250 \\
    %     GGIF [13]      & 32.491  & 0.9254 & 0.3361 \\
    %     Li20 [15]      & 28.238  & 0.8528 & 0.3317\\
    %     DeepFuse~\cite{ram2017deepfuse_short}  & 21.221  & 0.7291 & 0.3139 \\
    %     MEFNet [5]   &  \color{blue}32.973&  \color{blue}0.9680 & \color{blue}0.4683 \\
    %     Ours      & \color{red}33.092  & \color{red}0.9704 & \color{red}0.4742\\
        Methods & PSNR$\uparrow$ &  SSIM$\uparrow$ & Q$_\emph{C}$$\uparrow$ & MEF-SSIM$\uparrow$ \\\hline
        % &Mertens09~\cite{mertens2009exposure} &  Li13~\cite{li2013image}   &GGIF~\cite{kou2017multi} & Li20~\cite{li2020fast} &DeepFuse~\cite{ram2017deepfuse} &MEFNet~\cite{ma2019deep} & Ours \\
        % \hline
        % PSNR  & 27.981 & 20.043 & 29.451 & 26.320 & 20.122 & \color{blue}29.970 & \color{red}31.590  \\
        % SSIM &0.8515 & 0.8484 & 0.9093 & 0.8101 & 0.6562 & \color{blue}0.9604 & \color{red}0.9624 \\
        % Q$_\emph{C}$  & 0.3412 & 0.3250 & 0.3361 & 0.3317 & 0.3139 & \color{blue}0.4683 & \color{red}0.4742 \\
        % MEF-SSIM & 0.9126 & 0.8855 & 0.9472 & 0.9637 & 0.6892 & \color{blue}0.9637 & \color{red}0.9672 \\
        Mertens09 & 27.981 & 0.8515 & 0.3412 & 0.9126 \\
        Li13 & 20.043 & 0.8484 & 0.3250 & 0.8855 \\
        GGIF & 29.451&0.9093 &0.3361 &0.9472 \\
        Li20 & 26.320&0.8101&0.3317 &0.9637 \\
        DeepFuse &20.122 &0.6562 &0.3139 &0.6892 \\
        MEFNet &29.631 &0.9567 & 0.4548 & 0.9605 \\
        IFCNN & 29.970 &0.9597 &0.4574 & 0.9622 \\ 
        TransMEF & \color{blue}30.370 &\color{blue}0.9604 &\color{blue}0.4583 &\color{blue}0.9639 \\ 
        Ours &\color{red}31.590 &\color{red}0.9624 &\color{red}0.4683 &\color{red}0.9672 \\
    \bottomrule
\end{tabular}}
% \vspace{-2mm}
\caption{We quantitatively compare the performance of existing MEF methods when facing noisy inputs on our night dataset. The exposure number is set to $K=3$. Since DeepFuse~\cite{ram2017deepfuse} and TransMEF~\cite{qu2022transmef} takes 2 exposures only, we try several under- and over-exposed combinations, and choose the fused image that achieves the best performance for comparison. The best and 2nd best results are highlighted in {\color{red}red} and in {\color{blue}blue}, respectively. As seen, Ours beats the others in all metrics, achieving robustness under noises.}\label{table:noise_input_compare}
\vspace{-3mm}
\end{table}
% \vspace{-4mm}

\vspace{-2mm}
% \vspace{-2mm}
\paragraph{GFU vs. Bilinear upsampling.}\label{par:upsampling}
We compare GFU with bilinear upsampling to verify GFU's effectiveness. As seen in Tab.~\ref{table:diff_up}, performance gain is obtained by GFU over bilinear upsampling, while running time increase is also caused. For better performance, GFU is finally kept in our model. 

\paragraph{Noise inputs.} In this experiment, we show how our MEFLUT collaborates with other denoise approaches. We picked a night category of 30 cases with strong noise from our dataset to verify the robustness of our method under strong noisy inputs. Tab.~\ref{table:noise_input_compare} compares the performance when facing noises on our night dataset, where our fusion result is the best in all metrics. Fig.~\ref{fig:noise} shows a visual example, among which (a) is noisy inputs. (b) is our result without the denoise module, where our method remains robust in the presence of strong noisy inputs, achieving a high-quality fusion result. (c) is our result with denoise module~\cite{tomasi1998bilateral}, we can further apply an off-the-self denoise approach in practice to acquire a denoising image.

% We can further apply an off-the-shelf denoise approach~\cite{tomasi1998bilateral} in practice. 

% \subsubsection{Verification of Compatibility of Our Network to LUT.}
% % We verify the applicability of our network to 1D LUTs, we also use 1D LUTs for MEFNet to generates a weight map for fusion. 
% % In order to verify that the network we designed is more suitable for generating 1D LUTs, we use the same method to generate 1D LUTs for MEFNet~\cite{ma2019deep} and then use the generated 1D LUTs to perform the fusion task and the results are shown in Table.~\ref{table:validity}.
% % The results show that although MEFNet~\cite{ma2019deep} can use 1D LUTs to reconstruct the weight map for fusion, the metrics of it drop significantly, so our designed network has a better applicability to 1D LUTs.
% In order to verify that the network we propose is more compatible for 1D LUTs' generation, we apply the same idea to MEFNet~\cite{ma2019deep} and used the generated 1D LUTs to perform the fusion task instead. As seen in Table.~\ref{table:validity}, although MEFNet~\cite{ma2019deep} produces similar 1D LUTs to reconstruct the weight maps, its quality has a significant drop. It demonstrates that our network has a better compatibility to 1D LUTs' generation.

\paragraph{Hyper-parameter.}
 The number of branches for DISA and the resolution of the down-sampled inputs both have an impact on the performance of our method, so we verify the impact of these parameters.
 Tab.~\ref{table:mo_br} shows the the impact of these parameters, and we find that the increase of the number of the branches of the DISA obviously improves the performance, which is because that the receptive field becomes larger due to the increase of the dilation rate, but after increasing to a certain extent, more noise is introduced and decreases the PSNR, SSIM, Q$_C$ and MEF-SSIM scores. 
 We also verify the impact of different resolution of the down-sampled inputs. We find that as the resolution increases, the model focuses on more detailed areas and achieves higher performance, but when increasing to a certain extent, the performance is basically unchanged. So a fairly shallow and compact architecture, and reasonable resolution settings enable our method to achieve the best and the most balanced performance.
\begin{figure}[t]

\centering
% \vspace{-1mm}
\includegraphics[width=1.0\linewidth]{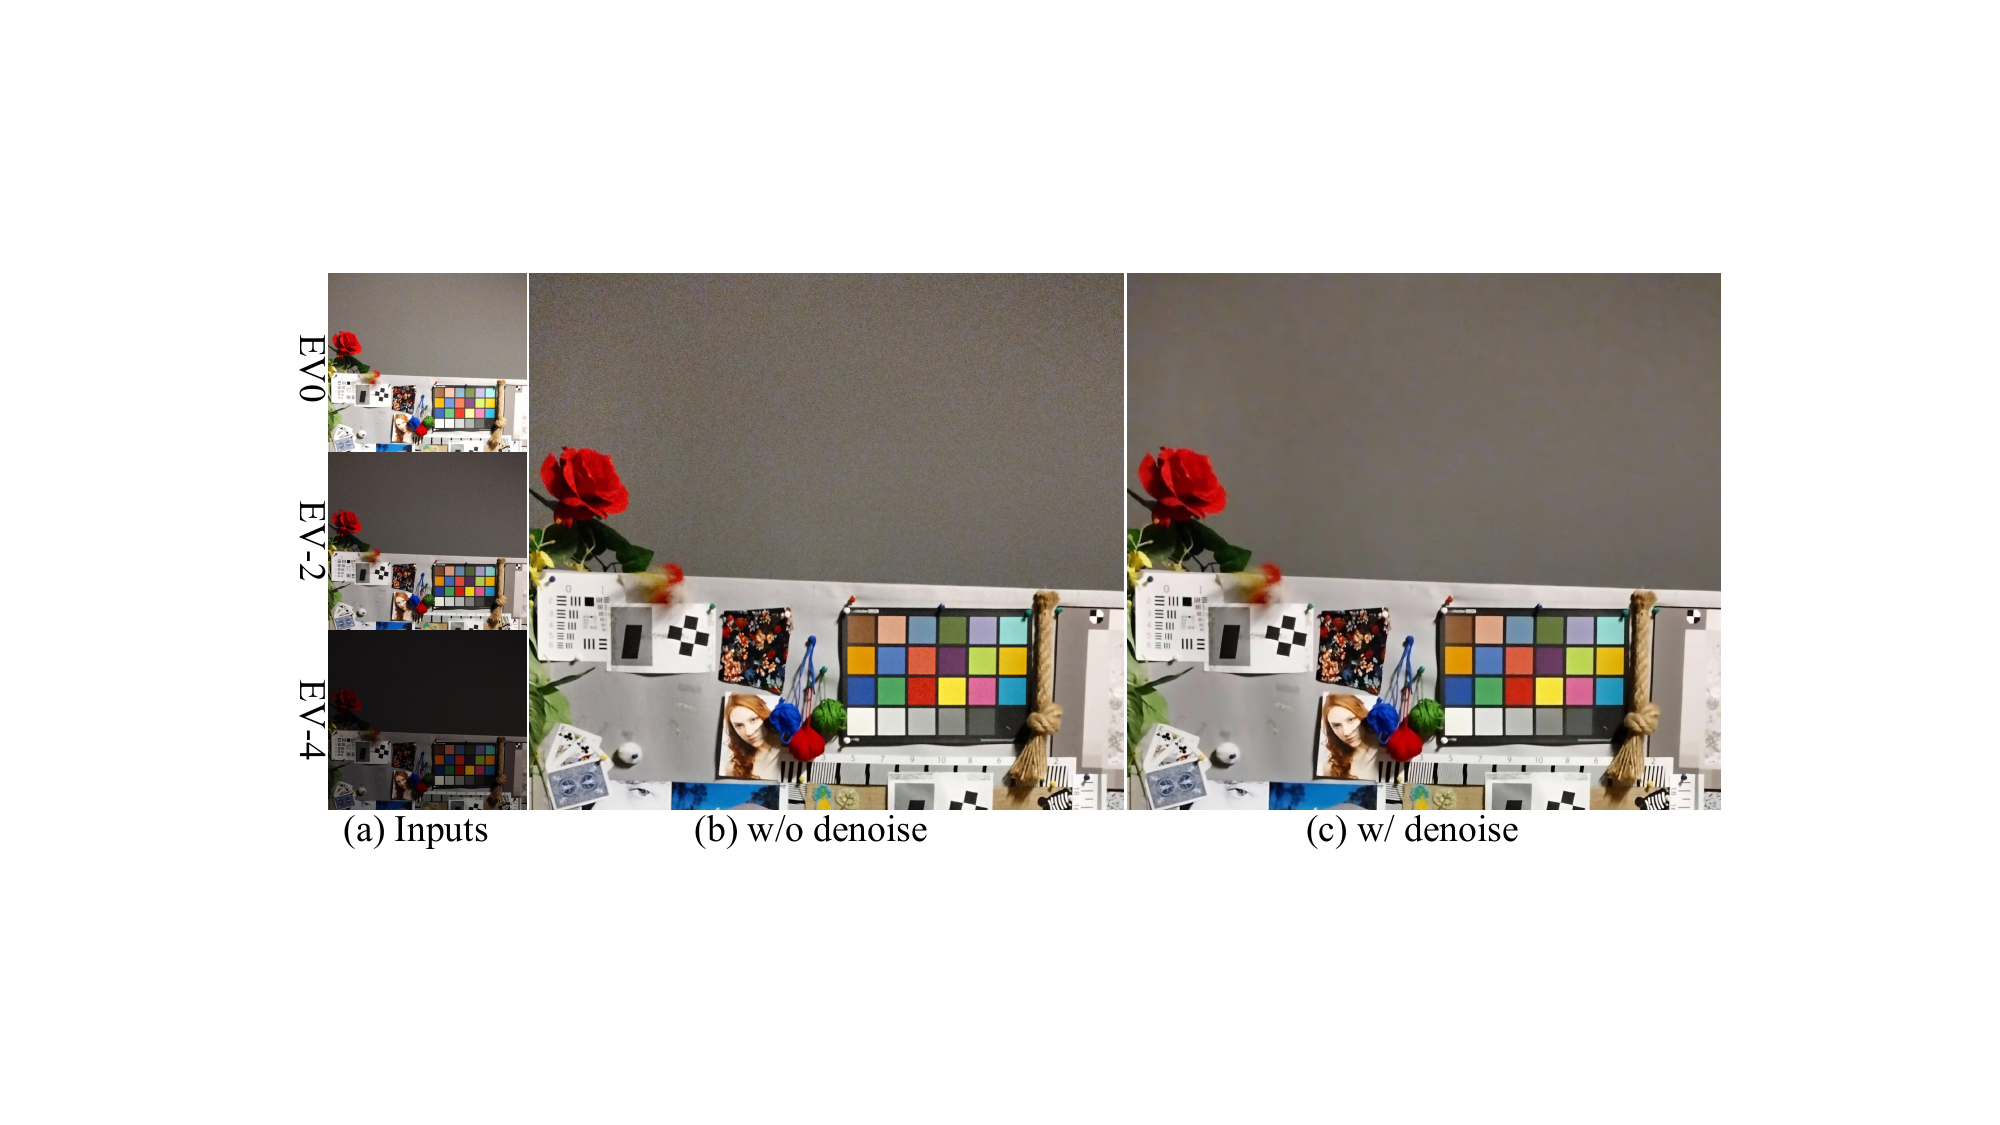}
\vspace{-5mm}
\caption{Our method works together with an image denoise approach. \textbf{Left}: inputs images with noise; \textbf{Middle}: our result without denoise; \textbf{Right}: our result with denoise.}
\vspace{-3mm}
\label{fig:noise}
\end{figure}

\begin{table}[t]
  \centering
  \resizebox{0.98\linewidth}{!}{
  \setlength{\tabcolsep}{9 pt}
  \vspace{-3mm}
  \begin{tabular}{c|cccc}
    \toprule %添加表格头部粗线
    Number of Branches & 2 & 3 & 4 & 5\\
    \hline
     PSNR$\uparrow$ & 30.117 & \textbf{31.387} & 30.016 & 28.633\\
     SSIM$\uparrow$ & 0.9570 & \textbf{0.9590} & 0.9578 & 0.9565\\
     Q$_C$ $\uparrow$ & 0.5913& \textbf{0.6075} & 0.5983 & 0.5927\\
     MEF-SSIM$\uparrow$ & 0.9682 & \textbf{0.9688} & 0.9681 & 0.9662\\
    \bottomrule
    Resolution & 32 & 64 & 128 & 256 \\
    \hline
     PSNR$\uparrow$ &  30.421  &30.569 & \textbf{31.387} & 31.383\\
     SSIM$\uparrow$ & 0.9560 & 0.9576 & \textbf{0.9590} & 0.9589\\
     Q$_C$ $\uparrow$ & 0.5989 & 0.6034 & \textbf{0.6075} & 0.6037 \\
     MEF-SSIM$\uparrow$ & 0.9667 & 0.9684 & \textbf{0.9688} & 0.9687\\
    \bottomrule
  \end{tabular}}
  % \vspace{-2mm}
  \caption{The impact of the number of branches of DISA, and the resolution of the down-sampled inputs. The exposure number is set to $K = 3$. The best results being highlighted in bold.}
  \label{table:mo_br}
  \vspace{-4mm}
\end{table}
\section{More Comparison with other Methods}
We compare our method with 8 previous MEF methods on our dataset and SICE, more comparison results are shown in \cref{fig:our_vis_su1,fig:our_vis4,fig:our_vis_su2,fig:sice_vis2}. 
As seen from them, the results of the other methods fail to recover details in the over-exposed area, while our method consistently recovers accurate contents with detail preservation.

\section{More Details of Our Dataset}
In the data collection stage, we collected more than 5000 image sequences with different exposure levels and scenes using 6 different commonly used brands of mobile phones. However, many of them contain distorted images or moving objects. We therefore conducted a difficult screening process to refine the dataset.
Sequences with significantly distorted performance (e.g., motion blur and out of focus) or obvious moving objects were discarded. As for those repeated sequences, we manually chose the most well-aligned one. For camera motion, we retained those sequences that had been successfully aligned by existing image registration algorithms~\cite{evangelidis2008parametric}.
After screening, a total of 960 static sequences are remained. The spatial resolution ranges from 12 to 16 mega-pixels. The collection is completed for over one month. Some sample sequences of this dataset are presented in Fig.~\ref{fig:sample_exp2}.
% We verify the impact of different regularization parameters $\lambda$ and the radius \emph{r} in the guided filter. A small $\lambda$ or \emph{r} can cause the weight map existing noise and dot artifacts, on the other hand a large $\lambda$ or \emph{r} can generate a smoother weight map but maybe cause loss of fine details. A reasonable parameter setting could make our method get better performance. As seen in Table.~\ref{table:mopa}, our default setting achieves the best performance.

% \subsection{Limitation and discussion}
% Although our method can achieve stable and efficient MEF across a variety of scenes, it has two limitations from 1D LUTs. First, our 1D LUTs currently only operates on the Y channel, which may not be good enough for color balance. One possible solution is to use the 1D LUTs on the UV channels as well but compatibility needs to be further investigated. Second, we query the 1D table pixel-wisely, causing the reconstructed weight map may be lack of smoothness and dot artifacts may appear as neighborhood information is not considered. Despite of GFU's smoothness capability on the weight map, its parameters cannot be adaptively set causing its uneven effects to various scenes, i.e. some are too dotted and some are over-smoothed resulting in Buddha light artifact. Two possible solutions include to learn a small model that provides more semantic information guidance for the 1D LUTs, and to learn a GFU with adaptive parameters. We leave them as our future work.

 \begin{figure*}[t]
   \centering
   \includegraphics[width=1.0\linewidth]{./Figs/ours_vis_su3_2_s.pdf}
   \caption{
  Qualitative comparison of the proposed method with (b) Mertens09~\cite{mertens2009exposure}, (c) Li13~\cite{li2013image}, (d) DeepFuse~\cite{ram2017deepfuse}, (e) MEFNet~\cite{ma2019deep}, (f) IFCNN~\cite{zhang2020ifcnn} and (g) TransMEF~\cite{qu2022transmef} on our test set. Input sequences with different exposures are shown in (a). The Zoomed red box region of the result shows that (h) our method hallucinate more reasonable details in saturated regions. Although (c) Li13 achieves considerable detail in saturated regions, unnatural artifacts appear.
%   Qualitative comparison on our test set. The Zoomed red box region of the result show that (h) our method hallucinate more reasonable details in saturated regions.
   } \label{fig:our_vis_su1}\vspace{-3mm}
 \end{figure*} 
 \begin{figure*}[t]
   \centering
   \includegraphics[width=1.0\linewidth]{./Figs/ours_vis_su3_3_s.pdf}
   \caption{
  Qualitative comparison of the proposed method with (b) Mertens09~\cite{mertens2009exposure}, (c) Li13~\cite{li2013image}, (d) Li20~\cite{li2020fast}, (e) DeepFuse~\cite{ram2017deepfuse}, (f) MEFNet~\cite{ma2019deep} and (g) TransMEF~\cite{qu2022transmef} on our test set. Input sequences with different exposures are shown in (a). The Zoomed red box region of the result shows that (h) our method hallucinates more reasonable details in saturated regions. Although (c) Li13 achieves considerable detail in saturated regions, unnatural gray artifacts appear.
%   Qualitative comparison on our test set. The Zoomed red box region of the result show that (h) our method hallucinate more reasonable details in saturated regions.
   } \label{fig:our_vis4}
 \end{figure*} 
\input{./include/fig-oursvis-su2.tex}
\begin{figure*}[htbp]
\centering
\includegraphics[width=1.0\linewidth]{./Figs/sice_vis_su_1_s.pdf}
\caption{
Qualitative comparison of the proposed method with (c) Mertens09~\cite{mertens2009exposure}, (e) Li13~\cite{li2013image}, (g) DeepFuse~\cite{ram2017deepfuse}, (i) MEFNet~\cite{ma2019deep}, (d) IFCNN~\cite{zhang2020ifcnn} and (f) TransMEF~\cite{qu2022transmef} on SICE~\cite{cai2018learning} dataset. Input sequences with different exposures are shown in (a) and (b). The zoom-in region of the red box shows that (h) our method contributes to a more natural image of the grasses with faithful details. Although (e) Li13 and (g) DeepFuse achieves considerable detail in saturated regions, (e) Li13 has unnatural artifacts, and (g) DeepFuse does not recover enough detail in dark area.
% Qualitative comparison on test set of SICE~\cite{cai2018learning}. The Zoomed red box region of the result show that (h) our method produces a more natural appearance with faithful detail and color reproduction.
} \label{fig:sice_vis2}
\end{figure*}

\begin{figure*}[h]
\begin{minipage}{1.0\linewidth}
\centerline{\includegraphics[width=\textwidth]{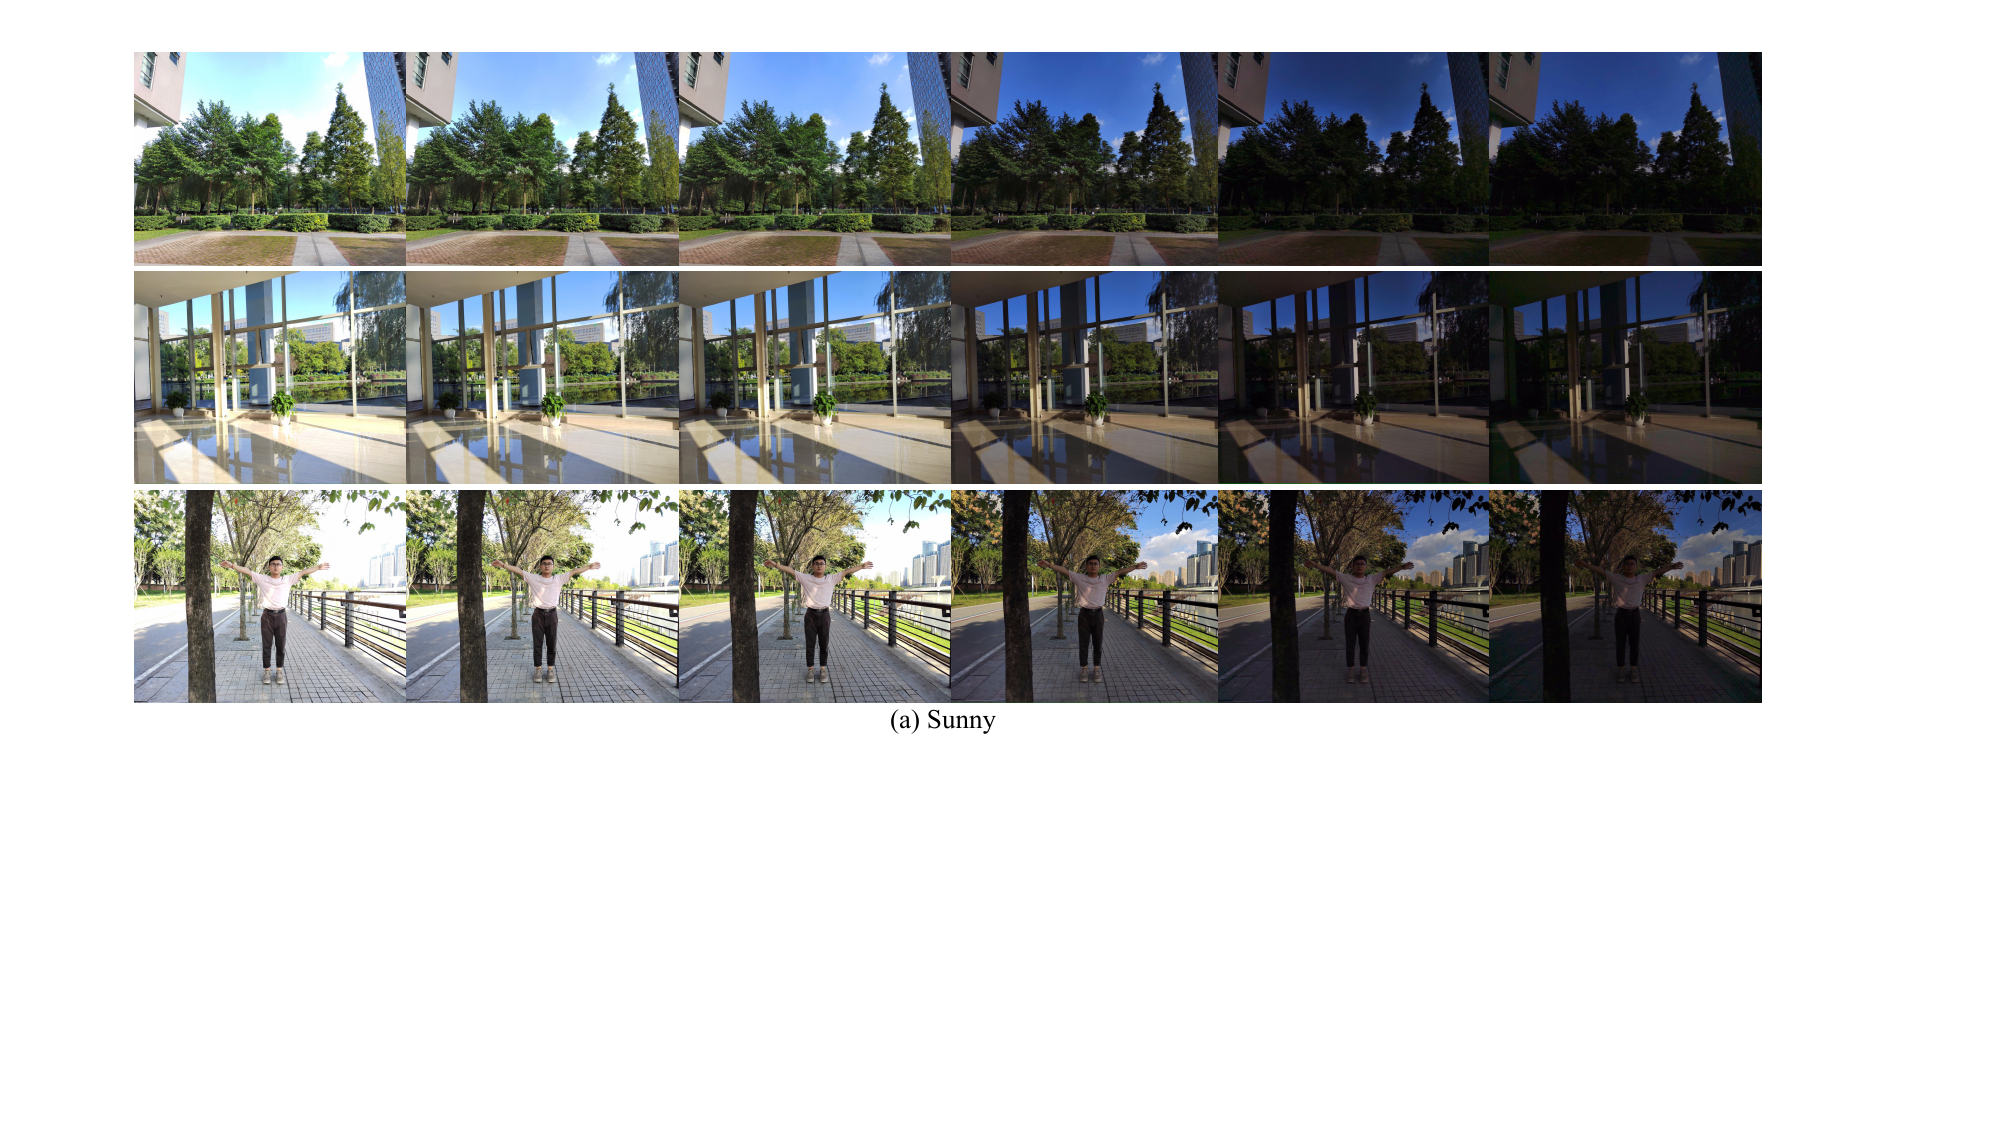}}
\centerline{\includegraphics[width=\textwidth]{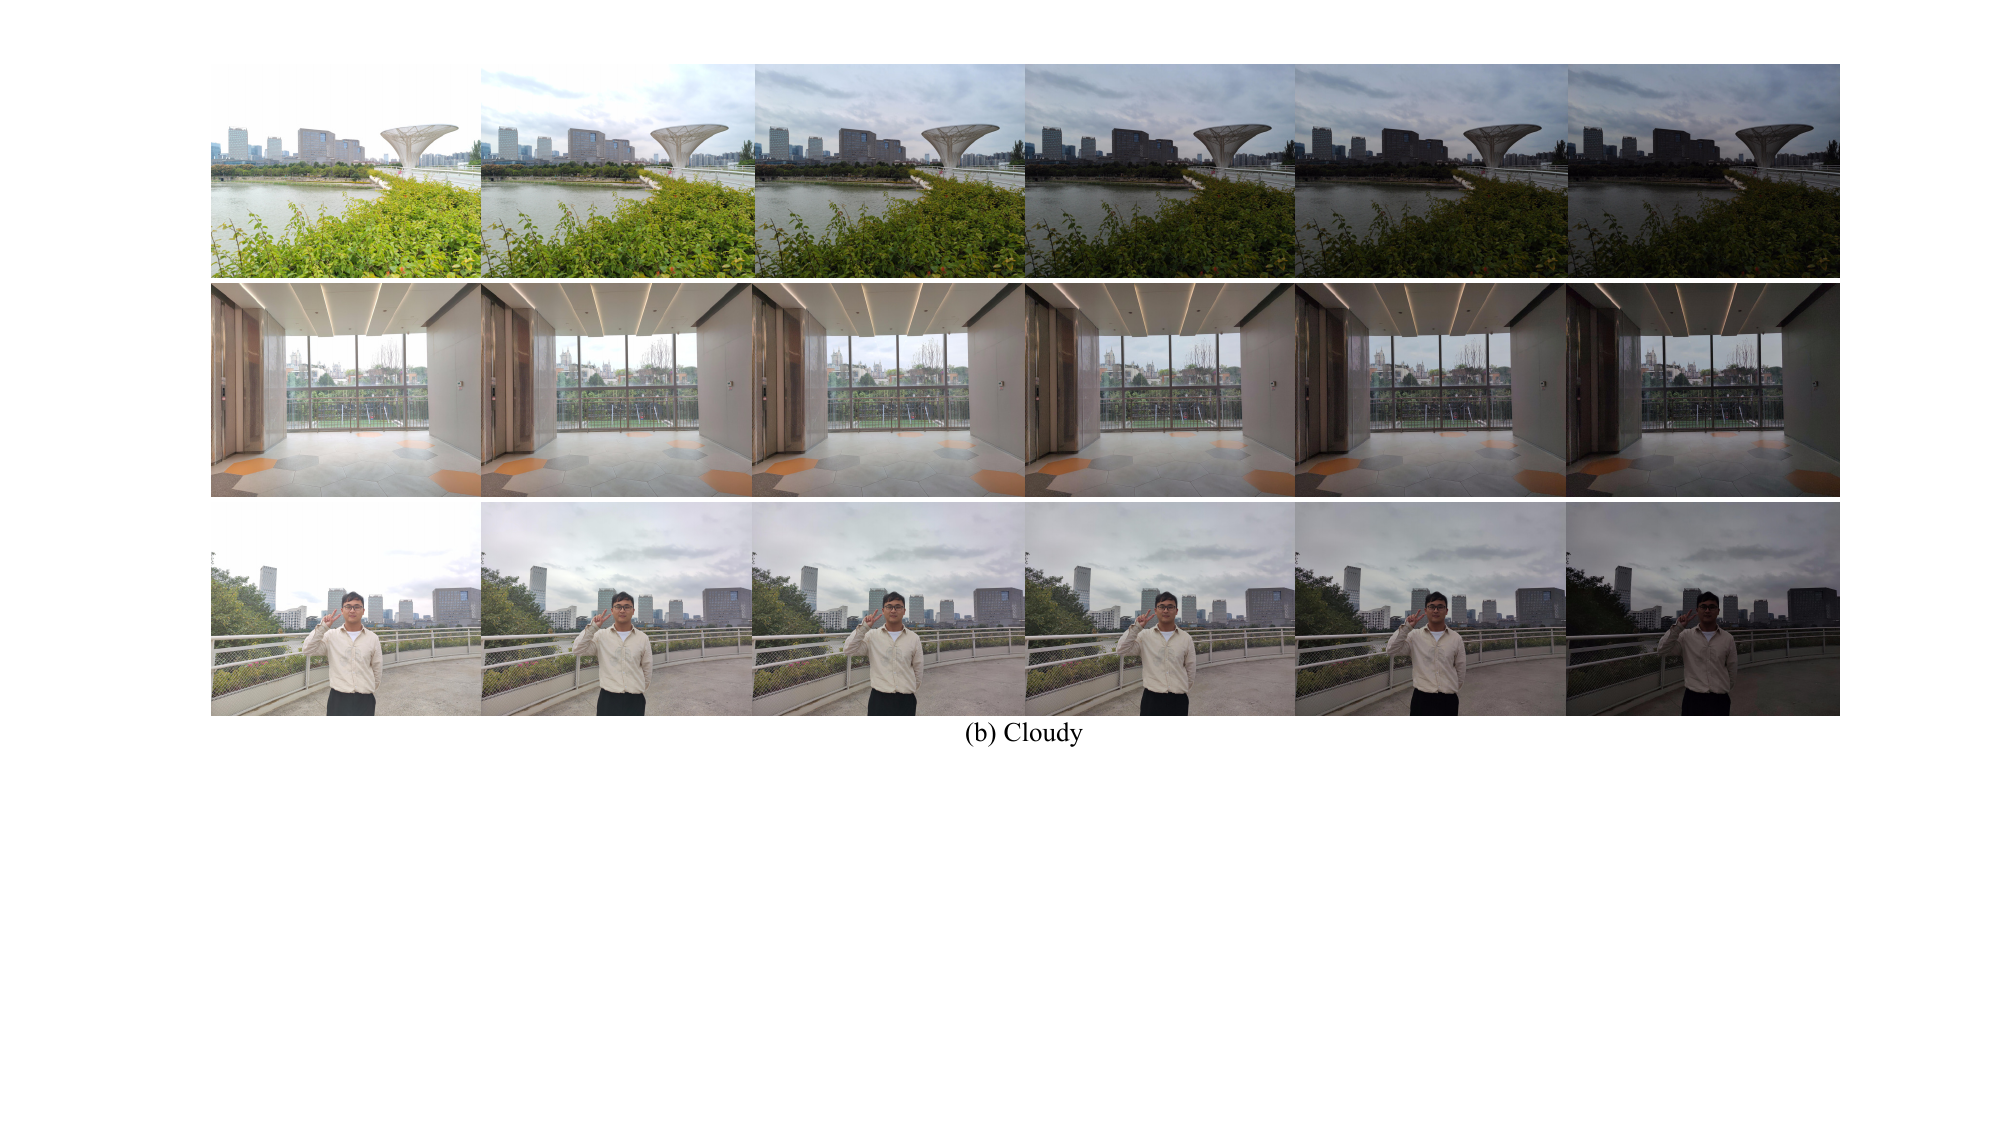}}
\centerline{\includegraphics[width=\textwidth]{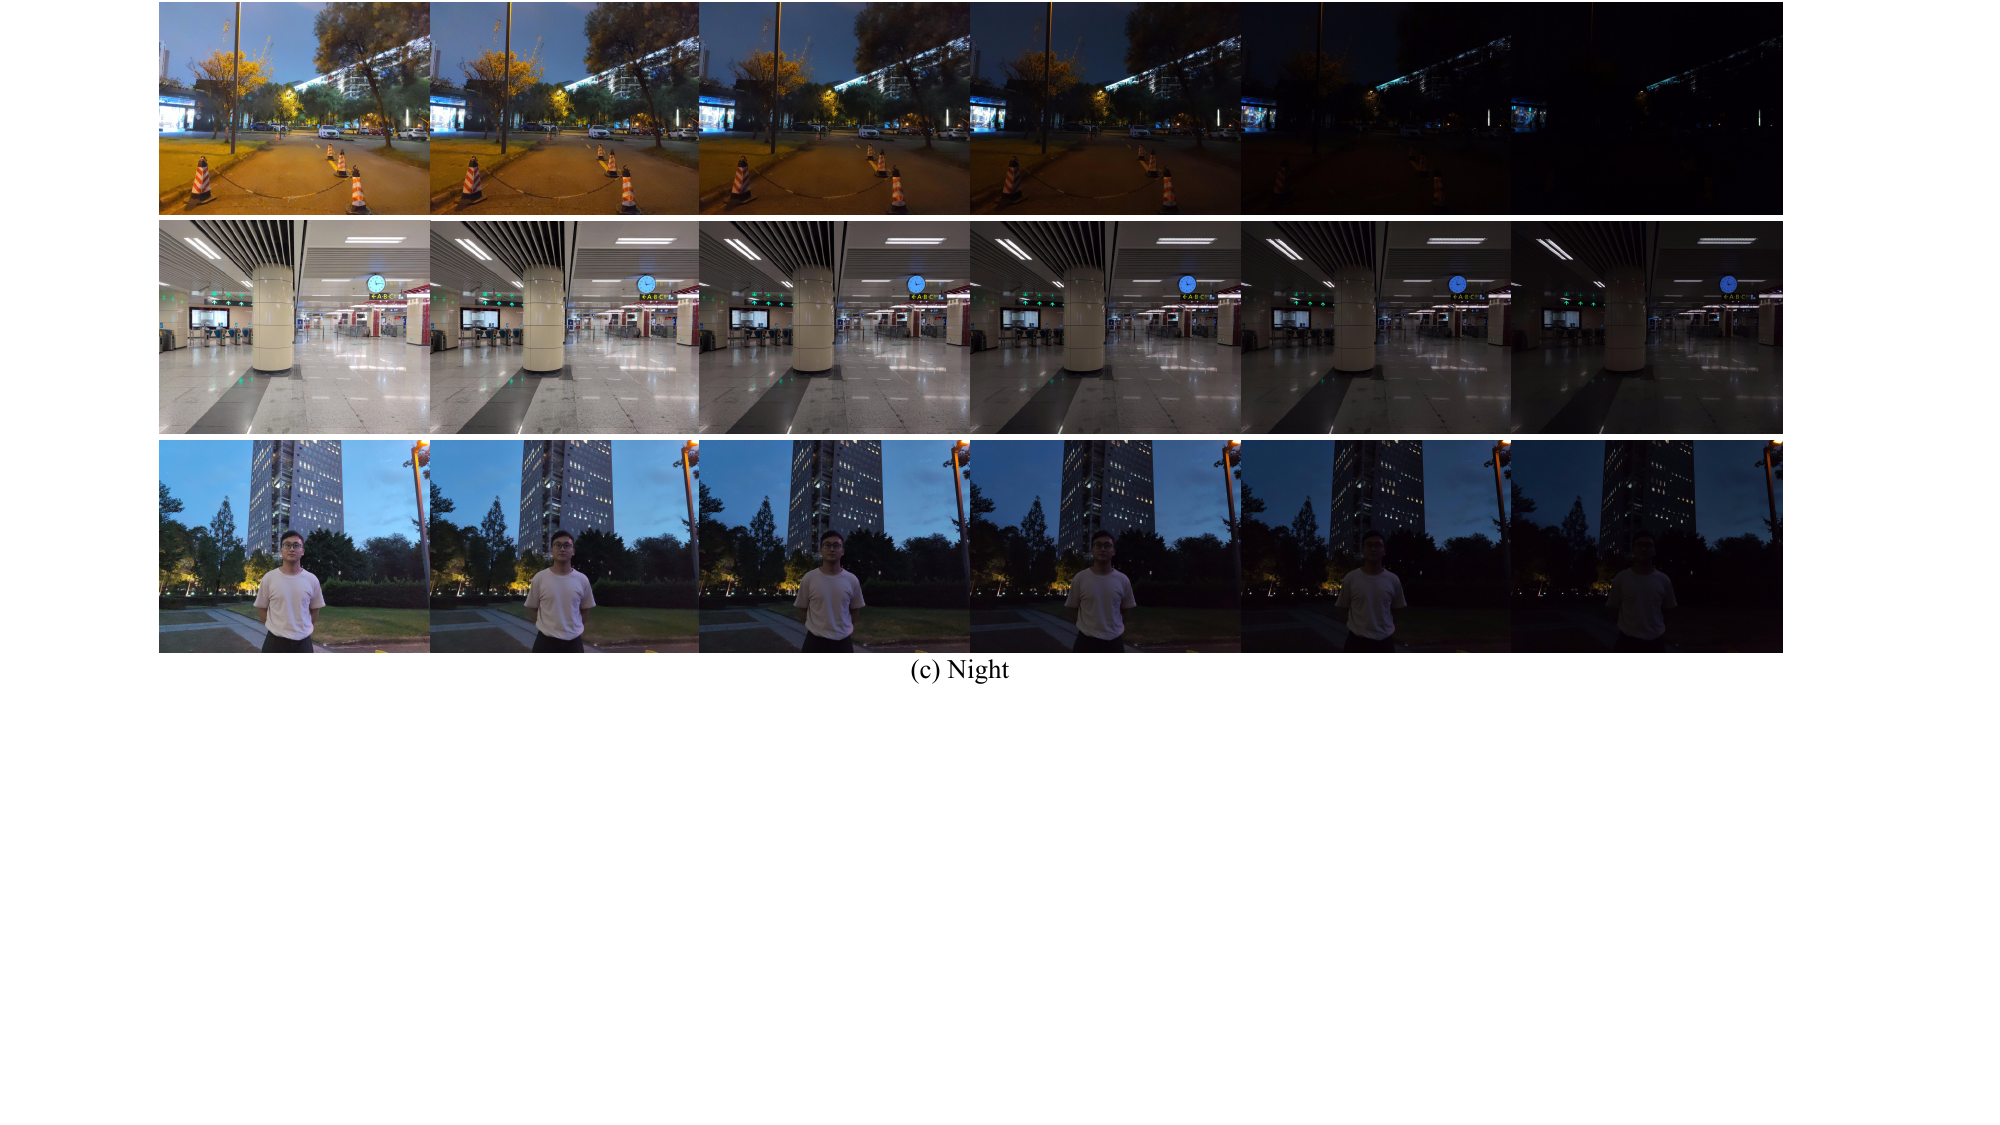}}
% \vspace{-0.37cm}
% \centerline{Image}
\end{minipage}
\caption{Sample source image sequences with different exposure levels in our dataset. We listed some scenes of (a) Sunny, (b) Cloudy, (c) Night. All data is collected by mobile phones.}
\label{fig:sample_exp2}
\end{figure*}
